# Supplementary material for: Propagation of wind-power-induced fluctuations in power grids
Source: arXiv:1809.09098 ancillary file (2019-05-10)
Supplement: Supplementary file 1 [file Supplemental_Material.pdf]

# Supplemental Material to "Propagation of wind-power-induced fluctuations in power grids"

Hauke Haehne,[1] Katrin Schmietendorf,[1] Samyak Tamrakar,[2] Joachim Peinke,[1,3] and Stefan Kettemann[2,4]

[1] *Institute of Physics and Forwind, Carl von Ossietzky Universität Oldenburg, Küpkersweg 70, 26129 Oldenburg, Germany*

[2] *Jacobs University, Department of Physics and Earth Sciences, Campus Ring 1, 28759 Bremen, Germany*

[3] *Fraunhofer IWES, Küpkersweg 70, 26129 Oldenburg, Germany*

[4] *Division of Advanced Materials Science, Pohang University of Science and Technology (POSTECH), San 31, Hyoja-dong, Nam-gu, Pohang 790-784, South Korea*

**CONTENTS**

Grid frequency measurements in the public power grid 3

Stochastic process for synthetic wind power production data 4

Linear Response Theory of power grids exposed to stochastic perturbations 6

Analytical derivation of frequency increment moments for a chain of nodes 9

References 11

## GRID FREQUENCY MEASUREMENTS IN THE PUBLIC POWER GRID

We measured the grid frequency at two locations in the public distribution grid, namely our own lab in Oldenburg (Küpkersweg 70, 26129 Oldenburg, Germany) as well as a lab at Max Planck Institute for Dynamics and Self-Organization in Göttingen (Am Fassberg 17, 37077 Göttingen, Germany). We used identical setups at both sites and data evaluation techniques originating from our earlier work [1]:

We took 10 kHz voltage samplings $u(t)$ of a single phase. Subsequently, we applied the method of *Instantaneous Frequency* (IF) [2] to estimate the frequency time series $f(t)$ from the sinusoidal voltage signal $u(t)$.

The IF reveals the dominant frequency component at each time instant $t$ and is thus suited for signals composed of one major frequency component. The method makes use of the fact that real-valued signals, such as the voltage signal $u(t)$, have conjugate symmetric Fourier representations, $\mathcal{F}[u](-\omega) = \mathcal{F}[u](\omega)^*$. Here, $\mathcal{F}$ denotes Fourier transform. The complex-valued analytic signal $z(t)$ is the inverse Fourier transform of the positive frequencies $\omega > 0$. Discarding the redundant negative frequency components makes the IF accessible. It is defined as the time derivative of the phase $\Phi(t)$ of the analytic signal $z(t)$:

$$f(t) = \frac{1}{2\pi}\frac{\mathrm{d}}{\mathrm{d}t}\Phi(t) = \frac{1}{2\pi}\frac{\mathrm{d}}{\mathrm{d}t}\arg(z(t)). \tag{S1}$$

In practice, $z(t)$ is obtained from the Hilbert transform $\mathcal{H}[u](t)$ of the original signal: $z(t) := u(t) + i\mathcal{H}[u](t)$. The Hilbert transform can be obtained from $\mathcal{H}[u](t) = (u * 1/\pi t')(t)$, where "$*$" denotes convolution.

To estimate the derivative in Eq. (S1) numerically, the phase $\Phi(t)$ was calculated for every time step in the voltage signal. Subsequently, the time derivative was estimated by linear fits of $\Phi(t)$ in disjoint blocks of 2000 samples. This procedure gives a frequency time series $f(t)$ with a time resolution of 200 ms. The $2\sigma$-confidence bounds of the linear fits are, in average, of size $\pm$ 1 mHz.

## STOCHASTIC PROCESS FOR SYNTHETIC WIND POWER PRODUCTION DATA

Power production time series $P(t)$ of renewable generators show certain statistic similarities to turbulence [3, 4]: We find long-range correlations and a characteristic Kolmogorov power spectrum $S(f)$ decaying with $f^{-5/3}$. Further, on small time scales $\theta$, the PDFs of increments $\Delta_\theta P(t) = P(t+\theta) - P(t)$ show heavy tails severely deviating from the Gaussian distribution. Such tails describe the increased probability of extreme fluctuations on short scales, an effect often referred to as *intermittency* in turbulence research [5].

In our numerical studies, we perturb the power grid with synthetically generated wind power feed-in time series which show the above-mentioned key properties. Such properties were shown to be essential for adequate modeling of frequency fluctuations induced by stochastic feed-in [6, 7]. To isolate the effect of perturbation spreading in our simulations, we use grids with no initial power, i.e. $P_i^0 = 0$ for all $i$, and perturb the system with signals $\delta P_j(t)$ at node $j$. We remark that all our results are as well applicable to grids with initial loads.

The dimensionless perturbation time series $\delta\Pi_j(t)$ is decomposed into a stochastic part $x(t)$ and an amplitude $\widehat{P}$ for which we chose $\widehat{P} = 1$ MW.

$$\delta\Pi_j(t) = \frac{J}{\gamma^2\omega_0}\widehat{P} \cdot x(t). \tag{S2}$$

The stochastic part $x(t)$ is obtained by means of the procedure introduced in [6]: First, a time series $\tilde{x}(t)$ is generated integrating the Langevin-type system of equations

$$\dot{y} = -\gamma y + \Gamma(t), \tag{S3}$$

$$\dot{\tilde{x}} = \tilde{x}\left(g - \frac{\tilde{x}}{x_0}\right) + \sqrt{D\tilde{x}^2}y, \tag{S4}$$

with $\gamma = 1.0$, $g = 0.5$, $x_0 = 2.0$ and $\Gamma$ being white Gaussian noise. The parameter $D$ serves to tune the degree of intermittency. Here we set $D = 2.0$, which corresponds to strongly intermittent noise.

In a next step, the resulting Fourier spectrum is modified so that the final power spectrum reproduces the Kolmogorov -5/3 decay: $S(f) \propto f^{-5/3}$. Transforming back to real space and normalization eventually yields $x(t)$.

We show a short part of the time series $\delta P_i(t)$ accompanied by the short-term increment PDF and power spectrum in Fig. S1. In the numerical simulations, we use a time step

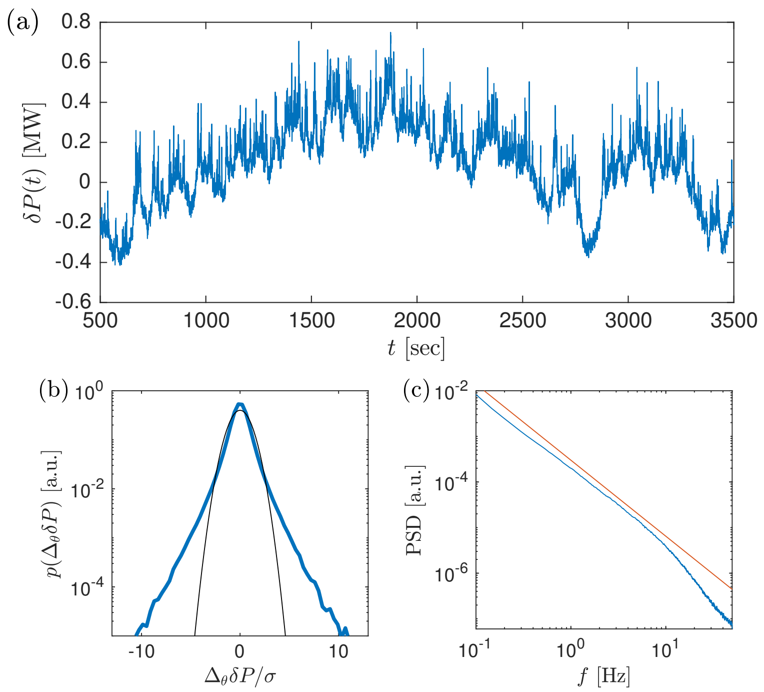


FIG. S1. **Synthetic wind power time series reproduce key stochastic features of real wind power generation data.** *(a)* Short part of synthetic time series $\delta P_j(t)$ used for the numerical investigations. *(b)* The PDF of short-term ($\theta = 0.01$ sec) increments $\Delta_\theta \delta P(t) = \delta P(t+\theta) - \delta P(t)$ shows severe deviations from the Gaussian distribution (black curve) in its tails. $x$-axis is plotted in units of the standard deviation $\sigma$ of increments $\Delta_\theta \delta P(t)$. *(c)* The power spectral density decays as $S(f) \propto f^{-5/3}$ (orange reference curve). This reproduces the characteristic Kolmogorov spectrum from turbulence.

$dt = 0.01$ sec and integrate the system with intermittent noise $\delta P_i(t)$ of length 19,800 sec with a Runge-Kutta scheme of order 4.

## LINEAR RESPONSE THEORY OF POWER GRIDS EXPOSED TO STOCHASTIC PERTURBATIONS

We start from the Swing Equation,

$$\tau^2 \ddot{\alpha}_i + 2\tau\dot{\alpha}_i = \frac{J}{\gamma^2\omega_0} P_i(t) - \sum_{j=1}^{N} \frac{J}{\gamma^2\omega_0} K_{ij} \sin(\vartheta_i^0 - \vartheta_j^0 + \alpha_i - \alpha_j), \tag{S5}$$

which models the deviations $\alpha_i(t) = \vartheta_i(t) - \vartheta_i^0$ of the phase $\vartheta_i(t)$ at node $i$ and time $t$ from the stable fixed point $\vartheta_i^0$. Here, $J$ is the inertia at each node, $\gamma = J/\tau$ is the damping constant and $\tau$ is the relaxation time scale. We consider time dependent production and consumption $P_i(t) = P_i^0 + \delta P_i(t)$, where the $P_i^0$'s correspond to the stable fixed point. For small deviations $|\alpha_i|$, we may linearize Eq. (S5) about the stable fixed point and find

$$\tau^2 \ddot{\alpha}_i + 2\tau\dot{\alpha}_i = -\sum_{j=1}^{N} \frac{J}{\gamma^2\omega_0} K_{ij} \cos(\vartheta_i^0 - \vartheta_j^0)(\alpha_i - \alpha_j) + \frac{J}{\gamma^2\omega_0} \delta P_i(t). \tag{S6}$$

We define the generalized Laplacian $\Lambda$ as

$$\Lambda_{ij} = -\frac{J}{\gamma^2\omega_0} K_{ij} \cos(\vartheta_i^0 - \vartheta_j^0) \quad \text{and} \quad \Lambda_{ii} = \frac{J}{\gamma^2\omega_0} \sum_j K_{ij} \cos(\vartheta_i^0 - \vartheta_j^0) \tag{S7}$$

and write

$$\tau^2 \ddot{\alpha}_i + 2\tau\dot{\alpha}_i + \sum_{j=1}^{N} \Lambda_{ij}\alpha_j = \frac{J}{\gamma^2\omega_0} \delta P_i(t). \tag{S8}$$

Further, we introduce $\delta\Pi_i(t) = J\delta P_i(t)/(\gamma^2\omega_0)$ to obtain

$$\tau^2 \ddot{\alpha}_i + 2\tau\dot{\alpha}_i + \sum_{j=1}^{N} \Lambda_{ij}\alpha_j = \delta\Pi_i(t). \tag{S9}$$

We now write the phase deviation $\alpha_i(t)$ as a generalized Fourier series by writing its time dependence as a Fourier integral and expanding its spatial dependence in terms of the eigenvectors $\boldsymbol{\phi}_n$ of the generalized Laplacian $\Lambda$, defined by $\Lambda\boldsymbol{\phi}_n = \Lambda_n\boldsymbol{\phi}_n$, where $\Lambda_n$ are its eigenvalues [8–10]. Thereby we obtain [9, 11]

$$\alpha_i(t) = \int_{-\infty}^{\infty} d\epsilon \sum_{n=0}^{N-1} c_n(\epsilon)\phi_{ni} e^{-\mathrm{i}\epsilon t}. \tag{S10}$$

Expanding the disturbance likewise in a generalized Fourier series we get

$$\delta\Pi_i(t) = \int_{-\infty}^{\infty} d\epsilon \sum_{n=0}^{N-1} \eta_n(\epsilon)\phi_{ni} e^{-\mathrm{i}\epsilon t}. \tag{S11}$$

Here, the Fourier components of the disturbance are defined by

$$\eta_n(\epsilon) = \int_{-\infty}^{\infty} \frac{dt'}{2\pi} e^{\mathrm{i}\epsilon t'} \sum_{i=1}^{N} \delta\Pi_i(t')\phi_{ni}^{*}. \tag{S12}$$

We now insert the expansions for $\alpha_i(t)$ and $\delta\Pi_i(t)$ into Eq. (S9) and find, requiring that the equation is fulfilled for each term of the Fourier series,

$$\left(-\tau^2\epsilon^2 - \mathrm{i}2\tau\epsilon + \Lambda_n\right) c_n(\epsilon) = \eta_n(\epsilon). \tag{S13}$$

For a given disturbance, the Fourier component of the phase deviation $c_n(\epsilon)$ is thus given in response to the one of the disturbance $\eta_n(\epsilon)$. Inserting that expression for $c_n(\epsilon)$ back into the Fourier series we get

$$\alpha_i(t) = \int_{-\infty}^{\infty} d\epsilon \sum_{n=0}^{N-1} \left(-\tau^2\epsilon^2 - \mathrm{i}2\tau\epsilon + \Lambda_n\right)^{-1} \eta_n(\epsilon)\phi_{ni}e^{-\mathrm{i}\epsilon t}. \tag{S14}$$

The integral over the angular frequency $\epsilon$ can be performed by means of the residuum theorem, noting that there are two poles in the lower complex plane, $\epsilon_{n\pm} = -\mathrm{i}(1 \pm \sqrt{1-\Lambda_n})1/\tau$. Inserting Eq. (S12) into Eq. (S14) yields

$$\alpha_i(t) = \int_{-\infty}^{\infty} d\epsilon \int_{-\infty}^{\infty} \frac{dt'}{2\pi} \sum_{n=0}^{N-1} (-\tau^2\epsilon^2 - 2\mathrm{i}\tau\epsilon + \Lambda_n)^{-1} \sum_{j=1}^{N} \delta\Pi_j(t')\phi_{nj}^{*}\phi_{ni}e^{\mathrm{i}\epsilon(t'-t)} \tag{S15}$$

$$= \int_{-\infty}^{t} \frac{dt'}{2\pi} \cdot (-2\pi\mathrm{i}) \sum_{n=0}^{N-1} \sum_{\pm} \frac{-1}{\tau^2} \cdot \frac{1}{\epsilon_\pm - \epsilon_\mp} \sum_{j=1}^{N} \delta\Pi_j(t')\phi_{nj}^{*}\phi_{ni}e^{\mathrm{i}\epsilon_\pm(t'-t)} \tag{S16}$$

$$= \int_{-\infty}^{t} dt' \sum_{n=0}^{N-1} \sum_{\pm} \frac{\mathrm{i}}{\tau^2(\epsilon_\pm - \epsilon_\mp)} e^{\mathrm{i}\epsilon_\pm(t'-t)} \sum_{j=1}^{N} \delta\Pi_j(t')\phi_{nj}^{*}\phi_{ni}. \tag{S17}$$

We have closed the integration path of $\epsilon$ clock-wise in the lower complex plane for $t' < t$. For $t' > t$, the path must be closed in the upper complex plane where no poles are present. Hence there are no contributions "from future" $(t' > t)$ to the integral. We remark that for $n = 0$, $\Lambda_0 = 0$ and hence $\epsilon_{0-} = 0$. Given that this pole lies on the real axis, its contribution must be multiplied with a factor 1/2. However, this contribution corresponds to a constant phase shift which does not impact the frequency $\omega_i(t)$ which we analyze in the following.

By replacing $\epsilon_\pm - \epsilon_\mp = \mp\frac{2\mathrm{i}}{\tau}\sqrt{1-\Lambda_n}$ we obtain the expression

$$\alpha_i(t) = \int_{-\infty}^{t} \frac{dt'}{\tau} \sum_{j=1}^{N} \delta\Pi_j(t')G_{ij}(t'-t) \tag{S18}$$

where the propagator $G_{ij}(t'-t)$ is defined by

$$G_{ij}(t'-t) = \sum_{n=0}^{N-1} \sum_{\sigma=\pm 1} \frac{\phi_{ni}\phi_{nj}^*}{2\sqrt{1-\Lambda_n}}(-\sigma) e^{(1+\sigma\sqrt{1-\Lambda_n})\frac{t'-t}{\tau}}. \tag{S19}$$

For the frequency $\omega_i(t) = \dot{\alpha}_i(t)$ we find

$$\omega_i(t) = \frac{d}{dt}\left[\int_{-\infty}^{t} \frac{dt'}{\tau} \sum_{j=1}^{N} \delta\Pi_j(t') G_{ij}(t'-t)\right] \tag{S20}$$

$$= \int_{-\infty}^{t} \frac{dt'}{\tau} \sum_{j=1}^{N} \delta\Pi_j(t') \partial_t G_{ij}(t'-t). \tag{S21}$$

We remark that the boundary terms are equal to zero because $G_{ij}(0)$ vanishes due to the summation over $\sigma = \pm 1$. For the $t$-derivative of the propagator we find

$$\partial_t G_{ij}(t'-t) = \sum_{n=0}^{N-1} \sum_{\sigma=\pm 1} \frac{\phi_{ni}\phi_{nj}^*}{2\sqrt{1-\Lambda_n}}(-\sigma) \cdot \left(-\left(\frac{1+\sigma\sqrt{1-\Lambda_n}}{\tau}\right)\right) e^{(1+\sigma\sqrt{1-\Lambda_n})\frac{t'-t}{\tau}} \tag{S22}$$

$$= \sum_{n=0}^{N-1} \sum_{\sigma=\pm 1} \frac{\phi_{ni}\phi_{nj}^*}{2\sqrt{1-\Lambda_n}} \left(\frac{\sigma}{\tau} + \frac{\sqrt{1-\Lambda_n}}{\tau}\right) e^{(1+\sigma\sqrt{1-\Lambda_n})\frac{t'-t}{\tau}}. \tag{S23}$$

To derive an expression for the variance of the frequency increment statistics $\langle \Delta_\theta \omega_i^2 \rangle$, we first evaluate Eq. (S21) at time $t+\theta$ and, subsequently, substitute $\hat{t} = t' - \theta$:

$$\omega_i(t+\theta) = \int_{-\infty}^{t} \frac{d\hat{t}}{\tau} \sum_{j=1}^{N} \delta\Pi_j(\hat{t}+\theta) \partial_t G_{ij}(\hat{t}-t). \tag{S24}$$

Therewith, the increment $\Delta_\theta \omega_i(t) = \omega_i(t+\theta) - \omega_i(t)$ follows as

$$\Delta_\theta \omega_i(t) = \int_{-\infty}^{t} \frac{dt'}{\tau} \sum_{j=1}^{N} \Delta_\theta \delta\Pi_j(t') \partial_t G_{ij}(t'-t). \tag{S25}$$

Finally, we focus on the case where a single node $j$ is driven by noise. We multiply Eq. (S25) with itself and apply an ensemble average $\langle \cdot \rangle$ over noise realizations to obtain

$$\langle \Delta_\theta \omega_i^2 \rangle = \int_{-\infty}^{t} \frac{dt'}{\tau} \int_{-\infty}^{t} \frac{dt''}{\tau} \langle \Delta_\theta \delta\Pi_j(t') \Delta_\theta \delta\Pi_j(t'') \rangle \, \partial_t G_{ij}(t'-t) \partial_t G_{ij}(t''-t). \tag{S26}$$

We find $\mathrm{acf}(|t'-t''|) := \langle \Delta_\theta \delta\Pi_j(t') \Delta_\theta \delta\Pi_j(t'') \rangle$, define $\delta := t' - t''$ and $\tilde{t} = t' - t$ and finally obtain

$$\langle \Delta_\theta \omega_i^2 \rangle = \int_{-\infty}^{0} \frac{d\tilde{t}}{\tau} \int_{\tilde{t}}^{\infty} \frac{d\delta}{\tau} \mathrm{acf}(|\delta|) \partial_t G_{ij}(\tilde{t}) \partial_t G_{ij}(\tilde{t}-\delta). \tag{S27}$$

## ANALYTICAL DERIVATION OF FREQUENCY INCREMENT MOMENTS FOR A CHAIN OF NODES

For the chain with open boundary conditions we find the eigenvalues of the generalized Laplacian to be $\Lambda_n = 2\Pi_K(1-\cos(k_n)) = 4\Pi_K \sin(k_n/2)^2$, for $n = 0,..,N-1$. Here, $\Pi_K = JK/(\omega_0\gamma^2)$ and $k_n = n\pi/N$. The eigenvectors $\boldsymbol{\phi}_n$ are $\phi_{0i} = 1/\sqrt{N}$ for $n = 0$ and $\phi_{ni} = \sqrt{2}/\sqrt{N}\cos(k_n(i-1/2))$, for $n = 1,..,N-1$.

We consider the case of large inertia $J$ when all nonzero eigenvalues are much larger than one, $\Lambda_n \gg 1$. Given that $\Lambda_1 = 4\Pi_K \sin^2(\pi/(2N)) \approx 4\Pi_K\pi^2/(4N^2)$ is the smallest nonzero eigenvalue, we find this condition fulfilled for $J \gg J_c = \omega_0\gamma^2N^2/(\pi^2K)$. In this regime, we approximate $\sqrt{1-\Lambda_n} \approx \mathrm{i}\sqrt{\Lambda_n}$. Inserting eigenvectors $\boldsymbol{\phi}_n$ and eigenvalues $\Lambda_n$ into the expression for the propagator $G_{ij}(t'-t)$, Eq. (S19), yields

$$\begin{aligned} G_{ij}(\Delta t = t-t') = & \frac{1}{N}\left(\frac{1}{2} - e^{-2\Delta t/\tau}\right) - e^{-\Delta t/\tau}\frac{1}{N\sqrt{\Pi_K}} \times \\ & \sum_{n=1}^{N-1} \frac{\cos\frac{\pi n(i-\frac{1}{2})}{N}\cos\frac{\pi n(j-\frac{1}{2})}{N}\sin\left(2\sqrt{\Pi_K}\sin(\frac{\pi}{2}\frac{n}{N})\frac{\Delta t}{\tau}\right)}{\sin(\frac{\pi}{2}\frac{n}{N})}. \end{aligned} \tag{S28}$$

For large $N \gg 1$ we can turn the summation in an integral over $x = n/N$ with $dx = 1/N$. Thus, we get

$$G_{ij}(\Delta t)|_{N\gg 1} = -\frac{e^{-\Delta t/\tau}}{\sqrt{\Pi_K}}\int_0^1 dx \frac{\cos\pi x(i-\frac{1}{2})\cos\pi x(j-\frac{1}{2})\sin\left(2\sqrt{\Pi_K}\sin(\frac{\pi}{2}x)\frac{\Delta t}{\tau}\right)}{\sin(\frac{\pi}{2}x)}. \tag{S29}$$

Noting that $0 < x < 1$, we further approximate $\sin(\frac{\pi}{2}x) \approx \frac{\pi}{2}x$ and perform the integrals to get

$$G_{ij}(\Delta t)|_{N\gg 1} = -\frac{e^{-\Delta t/\tau}}{\sqrt{\Pi_K}} g(i,j,\Delta t), \tag{S30}$$

where

$$\begin{aligned} g(i,j,\Delta t) = & \frac{1}{2\pi}\left(\mathrm{Si}[\pi(v\Delta t - i + j)] + \mathrm{Si}[\pi(v\Delta t + i - j)]\right) \\ & + \frac{1}{2\pi}\left(\mathrm{Si}[\pi(v\Delta t - i - j + 1)] + \mathrm{Si}[\pi(v\Delta t + i + j - 1)]\right). \end{aligned} \tag{S31}$$

$\mathrm{Si}(x) = \int_0^x \sin(y)/y\, dy$ is the Sine Integral. Further, we have introduced the velocity $v = \sqrt{\Pi_K}/\tau$.

In this article, we consider perturbations at one end of the chain, i.e. site $j = 1$. Hence, we need to know the propagator from site 1 to $i$. The function $g(i,1,\Delta t)$ turns out to be a step

function in $i-1-v\Delta t$ with only weak superimposed oscillations. Thus, we can approximate $g(i,1,\Delta t) \approx 1$ for $i-1 < v\Delta t$ and 0 otherwise, that is, it is a unit step down function. Inserting this into Eq. (S18), we find the change of phase in response to the perturbation at site $j=1$ to be

$$\alpha_i(t) = -\frac{1}{v\tau} \int\limits_{-\infty}^{t-(i-1)/v} \frac{dt'}{\tau} \delta\Pi_1(t') e^{-(t-t')/\tau}. \tag{S32}$$

Taking the time derivative we find for the frequency deviation at node $i$

$$\omega_i(t) = -\frac{1}{\tau}\alpha_i(t) - \frac{1}{v\tau^2}\delta\Pi_1(t-(i-1)/v)e^{-\frac{i-1}{v\tau}}. \tag{S33}$$

In this approximation, we find for the variance of the frequency increment statistics

$$\langle \Delta_\theta \omega_i^2 \rangle = \frac{1}{\tau^2}\langle \Delta_\theta \alpha_i^2 \rangle + \frac{2}{v\tau^3}\langle \Delta_\theta \alpha_i(t) \Delta_\theta \delta\Pi_1(t-(i-1)/v)\rangle e^{-\frac{i-1}{v\tau}} + \frac{1}{v^2\tau^4}\langle \Delta_\theta \delta\Pi_1^2 \rangle e^{-\frac{2(i-1)}{v\tau}}. \tag{S34}$$

The signal $\delta\Pi_1(t)$ we are perturbing the system with has a power spectral density $S(f) \propto f^{-5/3}$. Following Wiener-Khinchin theorem, we obtain for the variance of the increment statistics

$$\langle \Delta_\theta \delta\Pi_1^2 \rangle = c\theta^{2/3}. \tag{S35}$$

This allows us to calculate also the increments of frequency fluctuations and their moments: Inserting Eq. (S32) into Eq. (S34), we obtain for the second moment of the frequency increments

$$\langle \Delta_\theta \omega_i^2 \rangle = \frac{1}{\tau^2 \Pi_K} c\tau^{2/3} e^{-2\frac{i-1}{v\tau}} L(\theta/\tau), \tag{S36}$$

where the function $L(\theta/\tau)$ is given by

$$L(x=\theta/\tau) = x^{2/3} + 2\int_{-\infty}^{0} ds_1 \int_{-\infty}^{0} ds_2 e^{s_1+s_2}\left(|s_1-s_2|^{2/3} - |s_1-s_2-x|^{2/3}\right) + e^{-x}\int_0^x ds e^s s^{2/3} - 2\Gamma(5/3)(1-\cosh x). \tag{S37}$$

The integrals can be expressed in terms of incomplete Gamma-functions $\Gamma(5/3, x)$ as

$$L(x=\theta/\tau) = x^{2/3} + \frac{2\pi}{\sqrt{3}\Gamma(-2/3)}(e^{-x}-2) - e^x\Gamma(5/3,x) - 2\Gamma(5/3)(1-\cosh x). \tag{S38}$$

For $\theta/\tau < 1$, the leading order is $L(x = \theta/\tau) = x^{2/3} + 3/5x^{5/3} + O(x^2)$ and hence we find for $\theta < \tau$

$$\langle \Delta_\theta \omega_i^2 \rangle \approx \frac{1}{\tau^2 \Pi_K} \exp\left(-\frac{i-1}{\xi}\right) \langle \Delta_\theta \delta \Pi_1^2 \rangle \tag{S39}$$

$$\approx \frac{1}{JK\omega_0} \exp\left(-\frac{i-1}{\xi}\right) \langle \Delta_\theta \delta P_1^2 \rangle, \tag{S40}$$

where $\xi = \sqrt{JK}/(2\sqrt{\omega_0}\gamma)$.

At low inertia $J < J_c = \omega_0 \gamma^2 N^2/\pi^2 K$, there appear modes which decay more slowly with relaxation rates $\Gamma_n < 1/\tau$. Then, keeping only those slow decaying modes with $\Lambda_n < 1$, we find

$$G_{ij}(\Delta t = t - t' > \tau)|_N \approx \frac{1}{2N} - \sum_{\{n|0<\Lambda_n<1\}} \frac{\phi_{ni}\phi_{nj}^*}{2(1-\Lambda_n/2)} e^{-\frac{1}{2}\Lambda_n \frac{t-t'}{\tau}}. \tag{S41}$$

Approximating $\Lambda_n \approx \Pi_K a^2 k_n^2$ and using for large $N \gg 1$ the continuum approximation $k_n \to k$, we can perform the integral over $k$ and find

$$G_{i1}(\Delta t = t - t' > \tau)|_N \approx -\frac{1}{\sqrt{2\pi \Pi_K a^2 (t-t')/\tau}} \exp\left(-\frac{(i-1)^2}{2\Pi_K (t-t')/\tau}\right), \tag{S42}$$

which has the form of a diffusion propagator with diffusion constant $D = \Pi_K a^2/\tau$ [9],

$$G_{i1}(\Delta t = t - t' > \tau)|_N \approx -\frac{1}{\sqrt{2\pi D(t-t')}} \exp\left(-\frac{(i-1)^2 a^2}{2D(t-t')}\right). \tag{S43}$$

In the last step, we have introduced a spatial scale $a$, the length of a transmission line, to define the diffusion constant $D$ in the common way. However, we note that one could principally perform these calculations in terms of node indices as distance measure as before.

---


[1] H. Haehne, J. Schottler, M. Waechter, J. Peinke, and O. Kamps, EPL (Europhysics Letters) **121**, 30001 (2018).

[2] B. Boashash, Proc. IEEE **80**, 520 (1992).

[3] P. Milan, M. Wächter, and J. Peinke, Phys. Rev. Lett. **110**, 138701 (2013).

[4] M. Anvari, G. Lohmann, M. Wächter, P. Milan, E. Lorenz, D. Heinemann, M. R. R. Tabar, and J. Peinke, New J. Phys. **18**, 063027 (2016).

[5] M. Wilczek and R. Friedrich, Phys. Rev. E **80**, 016316 (2009).

[6] K. Schmietendorf, J. Peinke, and O. Kamps, Eur. Phys. J. B **90**, 222 (2017).

[7] S. Auer, F. Hellmann, M. Krause, and J. Kurths, Chaos **27**, 127003 (2017).

[8] T. Nishikawa and A. E. Motter, New J. Phys. **17**, 015012 (2015).

[9] S. Kettemann, Phys. Rev. E **94**, 062311 (2016).

[10] T. Coletta and P. Jacquod, Phys. Rev. E **93**, 032222 (2016).

[11] L. A. Torres-Sánchez, G. T. Freitas de Abreu, and S. Kettemann, under review, arXiv:1706.10130 (2017).
